# Supplementary material for: Tensorial Spin-Phonon Relaxation Reveals Mode-Selective Relaxation Pathways in a Single-Molecule Magnet
Source: arXiv:2507.17910 source file (2025-07-23)
Supplement: Supplementary file 1 [file Supplemental_Information.pdf]

# Supplemental Information for: Tensorial Spin–Phonon Relaxation Reveals Mode-Selective Relaxation Pathways in a Single-Molecule Magnet

Roman Dmitriev,[1] Nosheen Younas,[1,2] Yu Zhang,[2,a)] Andrei Piryatinski,[2,b)] and Eric R Bittner[3,c)]

[1)] *Department of Physics, University of Houston, Houston, Texas 77204, USA*

[2)] *Theoretical Division, Los Alamos National Laboratory, Los Alamos, New Mexico 87545, United States*

[3)] *Department of Chemistry, University of Houston, Houston, Texas 77204, USA*

[a)] Electronic mail: zhy@lanl.gov

[b)] Electronic mail: apiryat@lanl.gov

[c)] Electronic mail: ebittner@Central.UH.EDU

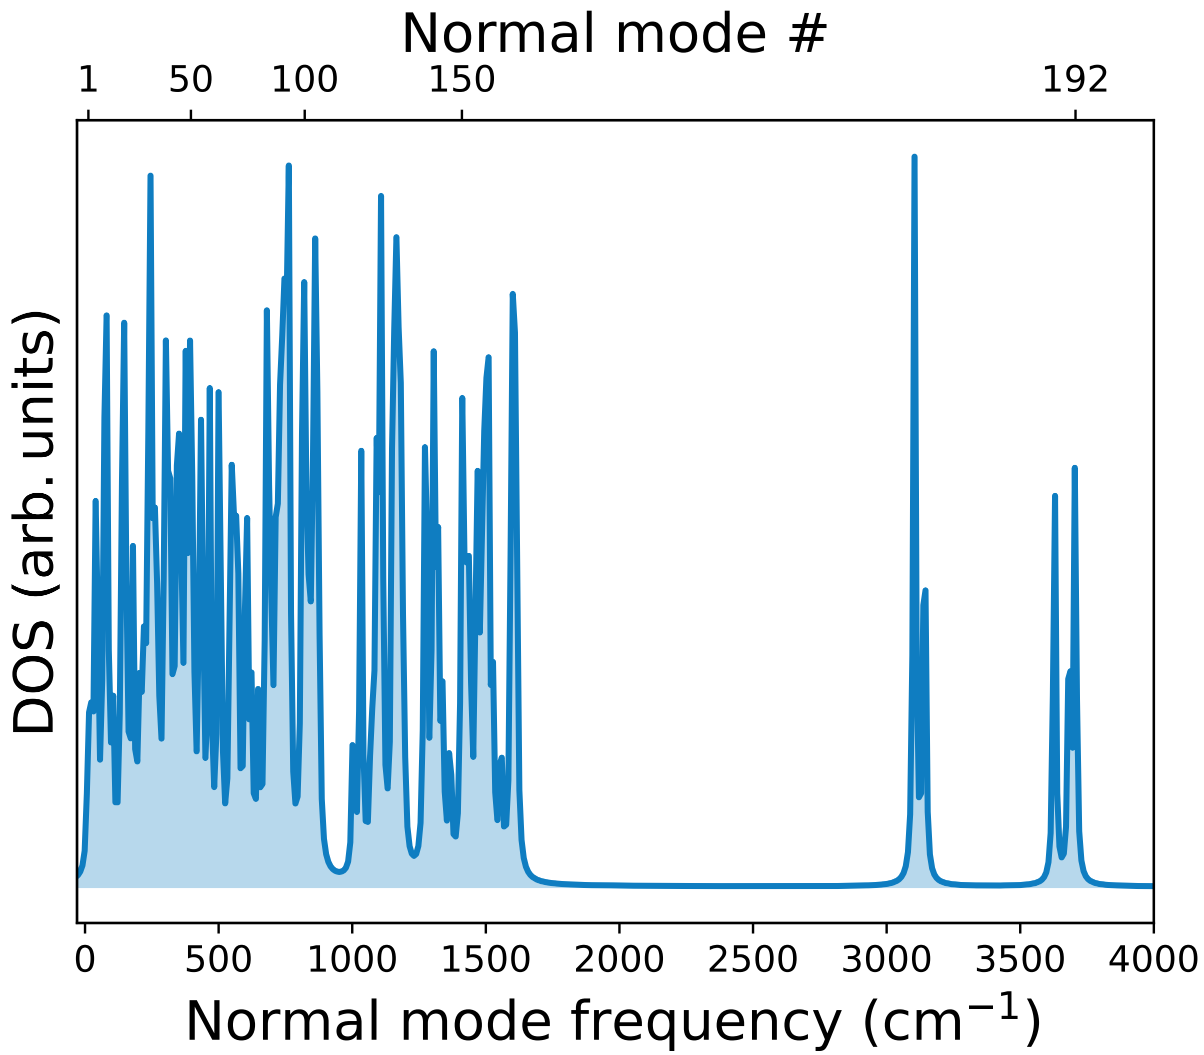


FIG. S1. Density of states of vibrational normal modes. Line broadening of 5 cm$^{-1}$ was introduced for visual clarity.

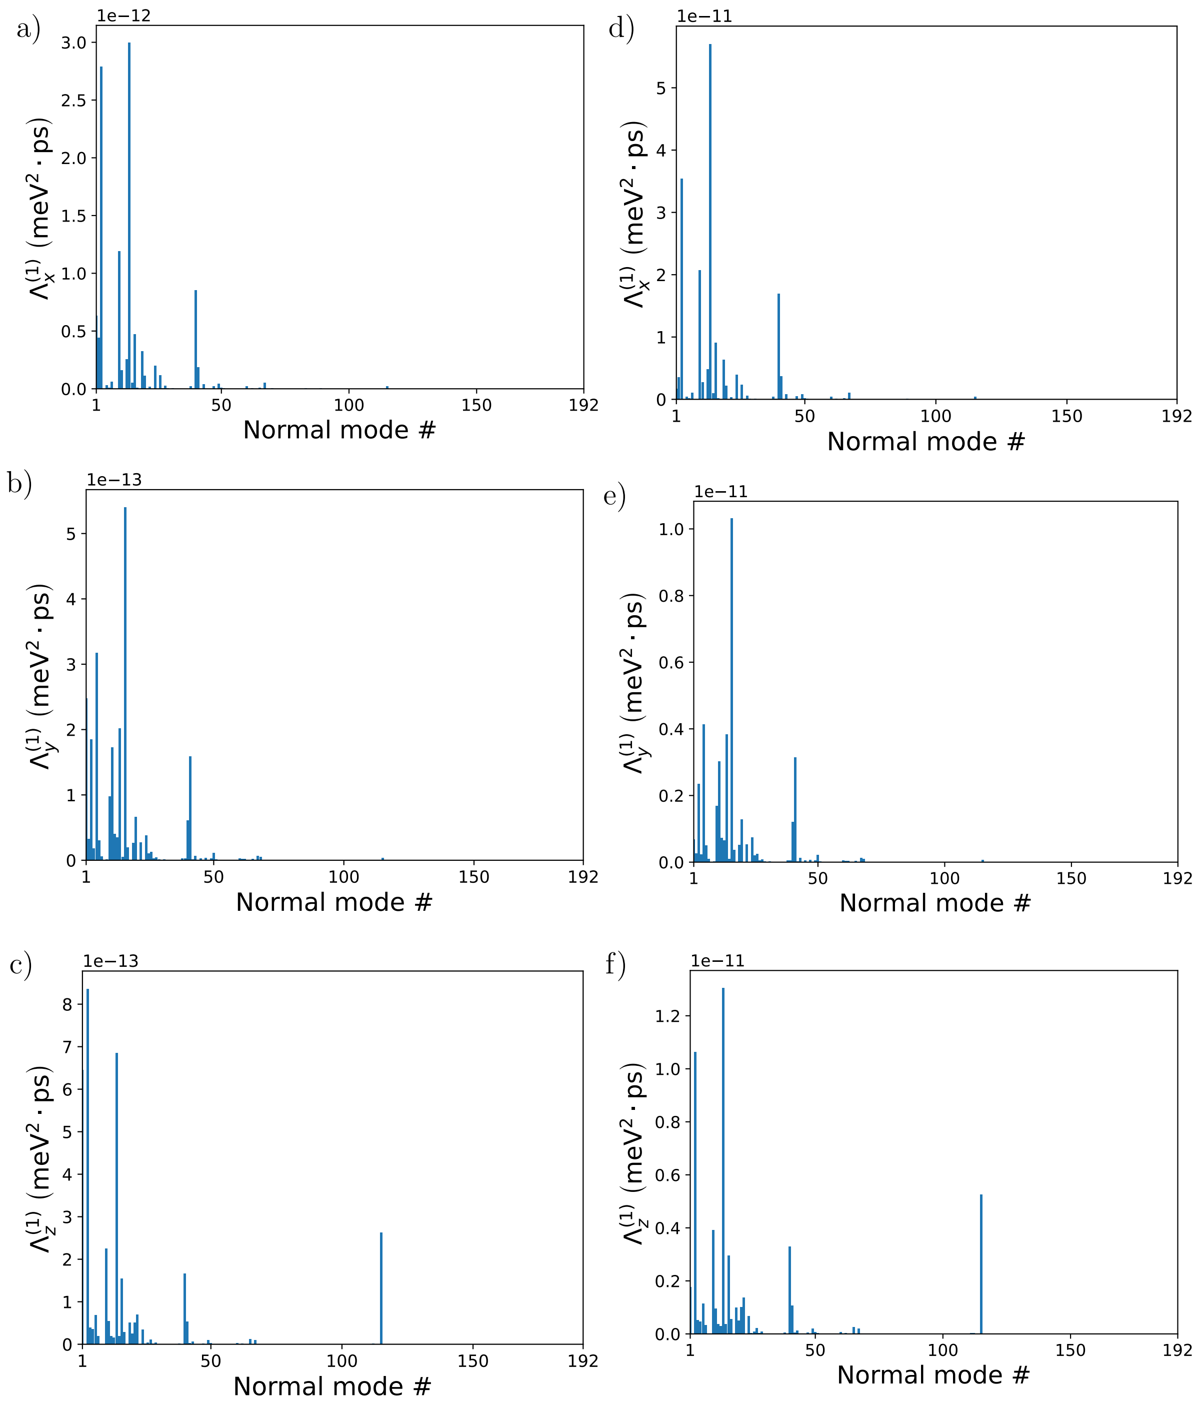


FIG. S2. Diagonal components of first order relaxation tensor $\Lambda^{(1)}$: (a − c) calculated with Lorentzian linewidth $\lambda_q = 2$ cm$^{-1}$; (d) − f)) calculated with Lorentzian linewidth $\lambda_q = 100$ cm$^{-1}$

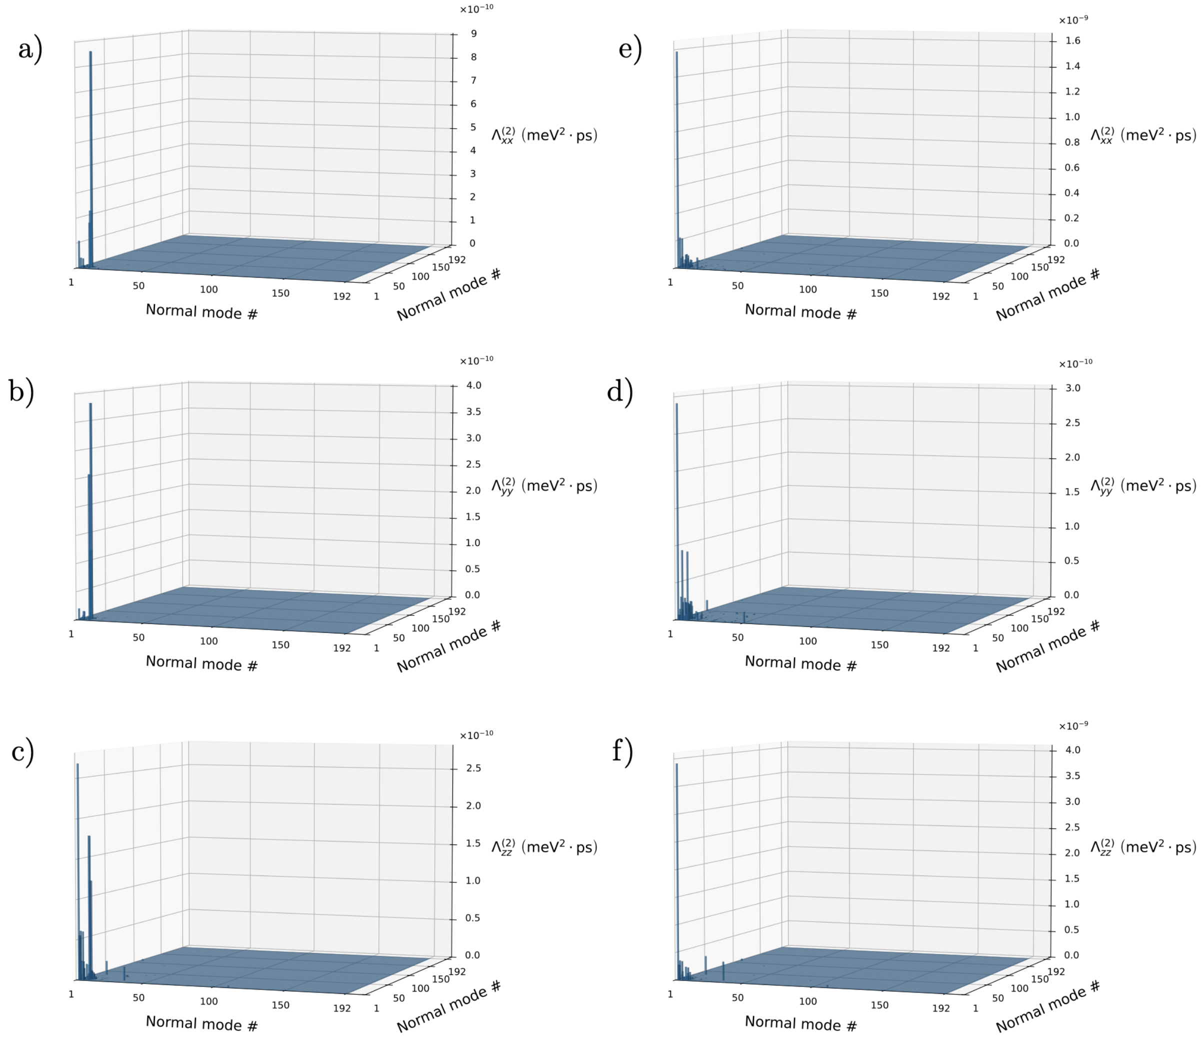


FIG. S3. Diagonal components of second order relaxation tensor $\Lambda^{(2)}$: (a – c) calculated with Lorentzian linewidth $\lambda_q = 2$ cm$^{-1}$; (d) -f)) calculated with Lorentzian linewidth $\lambda_q = 100$ cm$^{-1}$
